# Supplementary material for: Alleviating Matthew Effect of Offline Reinforcement Learning in Interactive Recommendation
Source: arXiv:2307.04571 source file (2023-07-10)
Supplement: Supplementary file 1 [file 06.appendix.tex]

% \clearpage
\appendix

\section{Proofs}
\label{appendix:proof}
We provide the proof for \mylemma{G_p}, which is adapted from the telescoping lemma in \cite{Algorithmic}.
\begin{proof}
    Let $W_j$ be the cumulative reward when we run policy $\pi$ on MDP $\widehat M$ for j steps and then on MDP $M$ for the next steps:
    \begin{equation*}
        W_j = \underset{\substack{a\sim\pi(\cdot|s_t)\\s_{t+1}\sim \widehat T(s_t,a_t), r\sim \widehat R(s_t,a_t), t<j\\s_{t+1}\sim T(s_t,a_t), r\sim R(s_t,a_t), t\ge j}}{\mathbb E}\Big[\sum_{t=0}^\infty\gamma^tr\Big].
    \end{equation*}
    Hence, $W_\infty=\eta_{\widehat{M}}(\pi),W_0=\eta_M(\pi)$, and we have a telescoping sum:
    \begin{equation*}
        \eta_{\widehat{M}}(\pi) - \eta_M(\pi) = \sum_{j=0}^\infty(W_{j+1}-W_j).
    \end{equation*}
    By definition, we can rewrite $W$ functions as:
    \begin{equation*}
        \begin{split}
            W_j &= R_{j-1}+\underset{s_j,a_j\sim\pi,\widehat{T}}{\mathbb E}\Big[\underset{r\sim R(s_j,a_j)}{\mathbb E}\gamma^j r + \underset{s_{j+1}\sim T(s_j,a_j)}{\mathbb E}\big[\gamma^{j+1}V_M^\pi(s_{j+1}) \big]\Big]\\
            W_{j+1} &= R_{j-1}+\underset{s_j,a_j\sim\pi,\widehat{T}}{\mathbb E}\Big[\underset{\hat r\sim \widehat R(s_j,a_j)}{\mathbb E}\gamma^j \hat r + \underset{\hat s_{j+1}\sim \widehat T(s_j,a_j)}{\mathbb E}\big[\gamma^{j+1}V_M^\pi(\hat s_{j+1}) \big]\Big]
        \end{split}
    \end{equation*}
where $$R_{j-1}=\underset{\substack{a\sim\pi(\cdot|s_t),\hat s_{t+1}\sim \widehat T(s_t,a_t), \hat r\sim \widehat R(s_t,a_t)}}{\mathbb E}\Big[\sum_{t=0}^{j-1}\gamma^t\hat r\Big].$$
So we have
\begin{equation*}
    \begin{split}
& W_{j+1} - W_j
=\ \gamma^{j}\underset{s_j,a_j\sim\pi,\widehat{T}}{\mathbb E}\Big[\underset{\hat r\sim \widehat R(s_j,a_j),\hat s_{j+1}\sim\widehat{T}(s_j,a_j)}{\mathbb E}\big[\hat r + \gamma V_M^\pi(\hat s_{j+1}) \big]\\
& - \underset{r\sim R(s_j,a_j),s_{j+1}\sim T(s_j,a_j)}{\mathbb E}\big[r + \gamma V_M^\pi(s_{j+1}) \big]\Big] = \ \gamma^{j} \underset{s_j,a_j\sim\pi,\widehat{T}}{\mathbb E}\big[G_{\widehat M}^\pi(s,a)\big].
    \end{split}
\end{equation*}
Then
\begin{equation*}
    \begin{split}
        & \eta_{\widehat{M}}(\pi) - \eta_M(\pi) 
        = \sum_{j=0}^\infty(W_{j+1}-W_j)\\
        &= \sum_{j=0}^\infty\gamma^{j} \underset{s_j,a_j\sim\pi,\widehat{T}}{\mathbb E}\big[G_{\widehat M}^\pi(s,a)\big]
        = \mathbb{E}_{(s,a)\sim\rho_{\widehat T}^\pi}\big[G_{\widehat M}^\pi(s,a)\big].
    \end{split}
\end{equation*}
\end{proof}
